# Supplementary material for: Droplet breakup driven by shear thinning solutions in a microfluidic T-Junction
Source: arXiv:1610.07800 ancillary file (2018-01-27)
Supplement: Supplementary file 1 [file TJ_fz10012_supmat_FINAL_03.pdf]

# Droplet breakup driven by shear thinning solutions in a microfluidic T-junction: Supplemental Material (SM)

Enrico Chiarello,[1] Anupam Gupta,[2,*] Giampaolo Mistura,[1] Mauro Sbragaglia,[2,†] and Matteo Pierno[1,‡]

[1] *Dipartimento di Fisica e Astronomia "Galileo Galilei" - DFA, Università di Padova, Via F. Marzolo 8, 35131 Padova, Italy*

[2] *Dipartimento di Fisica and INFN, Università di Roma 2 "Tor Vergata", Via della Ricerca Scientifica 1, 00133 Roma, Italy*

## I. FABRICATION OF THE MICROFLUIDIC T-JUNCTION

The microfluidic T-junction is made in PDMS (Polydimethylsiloxane, Sylgard 184, Dow Corning) using standard photo-lithography and replica-molding [1, 2] performed in a Class-V Clean Room: the master is realized in SU-8 (2050, MicroChem Corp.) on a silicon substrate by means of UV photolitography through a high resolution mask (4000 DPI) featuring the desired geometry: the two branches of the T-junction are designed to have the same rectangular cross section $W \times H$, with a width $W \approx 150$ $\mu m$ and a height $H \approx 100$ $\mu m$. The resulting master is casted in PDMS to obtain many replicas of the microchannels (Fig. 1-A in the manuscript). Each replica is then closed by oxygen plasma activated bonding [3] on a microscope glass and provided with Teflon tubings (internal diameter of 0.32 mm, TW30 Standard Wall Sleeve, Adtech). Finally, the internal walls are chemically functionalized: right after the plasma bonding, a solution of either 5% PVP/Water (Polyvinylpyrrolidone K90, AppliChem) or 1mM OTS/Hexadecane (Octadecyltrichlorosilane, Sigma Aldrich) is slowly flowed (at $\approx 1\mu$L/min) through the microchannels with a syringe-pump for about 30 minutes, after which they are flushed with distilled water and dried out with compressed air [4]. As a result, either the PDMS or glass walls are coated with a thin permanent hydrophilic (PVP) or hydrophobic (OTS) layer of molecules, allowing to use an aqueous or oil continuous phase, respectively, with no wettability issues.

## II. EXPERIMENTAL SETUP

The two inlets of the main and the side branches of the microfluidic T-junction are coupled by Teflon tubing to two glass syringes (SGE Analytical Sciences), while the outlet tubing goes to a reservoir at atmospheric pressure. The flow rate $Q_d$ of the dispersed phase and the flow rate $Q_c$ of the continuous phase are controlled by two independent syringe-pumps (PHD 2000, Harvard Apparatus). It is thus possible to vary the flow-rate ratio $\varphi$, defined as the ratio between $Q_d$ and $Q_c$:

$$\varphi = \frac{Q_d}{Q_c}. \tag{1}$$

The acquisition system is an improved version of the one used in a previous work [4]. A custom made software controls the pumps and a high speed Camera-Link CMOS camera (EoSens CL MC1362, Mikrotron) coupled to an inverted microscope (Eclipse Ti-E, Nikon), which acquires images of the droplets. The same software analyzes the images in a region of interest far downstream of the T-junction (Fig. 1-A in the manuscript) where the droplets are fully formed. All the droplets crossing this region are tracked, measuring quantities such as the droplets length $L$, velocity $u$ and the time interval $T$ between consecutive droplets in real-time (up to $\approx 1000$ fps). It thus allows to acquire quantitative information for a large amount of droplets in limited time and storage space, reducing the number of saved images to be just enough to cover a few full droplet breakups, for offline qualitative analysis. More importantly, it allows to monitor whether the droplets production has reached stability (i.e. the average droplet size has become constant in time) before starting to collect data. By using glass syringes and Teflon tubing, the elasticity in the system is reduced to a minimum. Indeed, after switching off the syringe pumps, the droplets in the microchannels are observed to stop immediately.

**Procedures**. The experiments are carried out by fixing the flow rate ratio $\varphi = Q_d/Q_c$ and by slowly varying the flow rate of the continuous phase $Q_c$. After each change in $Q_c$, the whole system is given enough time to stabilize. The

* present address: Mechanical Science and Engineering, University of Illinois, 1206 W. Green Street, Urbana, IL 61801, USA
† sbragaglia@roma2.infn.it
‡ matteo.pierno@unipd.it

time required to reach stability ranges from a few seconds at the highest flow rates to some minutes at the lowest flow rates. Only when the system has reached full stability, data are collected for at least a hundred consecutive droplets. Following this procedure, data are found to be highly reproducible and no hysteresis effects are found increasing or decreasing $Q_c$.

**Volume of the droplets**. The volume of the droplets in an ideal thread of equally spaced identical droplets can be computed from the frequency of droplets $f$ by the relation $V = Q_d/f$. This can be estimated using the measured time interval between consecutive droplets $\tau$, by the relation $V = Q_d\langle\tau\rangle$. This usually works reasonably well, but at very high flow rates it becomes difficult to measure $\tau$ due to the overall speed limitation of the acquisition system (camera and software). At very low flow rates the same $\tau$ has a large error, due to limitations of the syringe-pumps and the overall microfluidic system. Furthermore, estimating the droplet polydispersity is not a simple task [5].

**Length of the droplets** We therefore opt to use the average normalized droplet length $L/W$ (and corresponding error) to estimate the droplet size, as it is directly measured from the images and makes a direct estimation of the droplet polydispersity possible. More precisely, the average length is estimated by the median of the lengths, which is not affected by the outliers (faulty data that have to be discarded) which, due to image processing and tracking failure, are sometimes present when the acquisition system is driven to the highest speeds. Correspondingly, for the same reason, the error is computed by the Inter Quartile Range (IQR).

**Swelling** The normalization by the channel width $W$ for the droplet length is the same for all the experiments, with the exception of the ones employing hexadecane as continuous phase. Swelling of PDMS due to hexadecane caused a $\approx 10\%$ reduction in $W$ and $H$. However, the normalization is performed with the proper value of $W$ measured at the time of the experiment, and not the nominal one. The same is true for geometrical parameters in the Capillary number Ca.

## III. EFFECTIVE CAPILLARY NUMBER

For a Newtonian fluid with constant dynamic viscosity $\eta_c$, flowing in a channel with an average velocity $U_{av}$, the Capillary number Ca is defined by:

$$\mathrm{Ca} = \frac{\eta_c U_{av}}{\sigma}. \tag{2}$$

Within a shear thinning continuous phase, the Capillary number can be defined in terms of an effective (shear dependent) viscosity $\eta_c(\dot\gamma_{\mathrm{eff}})$ [6]

$$\mathrm{Ca}_{\mathrm{eff}} = \frac{\eta_c(\dot\gamma_{\mathrm{eff}}) U_{av}}{\sigma}. \tag{3}$$

Operatively, the effective shear rate $\dot\gamma_{\mathrm{eff}}$ scales linearly with the average velocity $U_{av}$ and is inversely proportional to the characteristic lengthscale $\delta$

$$\dot\gamma_{\mathrm{eff}} = \frac{3U_{av}}{\delta}. \tag{4}$$

The characteristic lengthscale $\delta$ is set to $W$ in our study (see text for further comments). The numerical prefactor 3 is fixed in such a way that for a Newtonian fluid driven by a pressure gradient $\nabla P$ between two (no-slip) parallel plates at distance $\delta$, the definition (4) coincides with the average shear rate developed in the system. Indeed, for such a simple fluid, we have the velocity profile $u_x(y) = (|\nabla P|/2\eta_c)y(\delta - y)$, resulting in an average velocity $U_{av} = 2\int_0^{\delta/2} u_x(y)\,dy/\delta = |\nabla P|\,\delta^2/12\eta_c$. The corresponding shear rate is $\dot\gamma = (|\nabla P|/2\eta_c)(\delta - 2y)$, and its averaged value is $2\int_0^{\delta/2} \dot\gamma\,dy/\delta = |\nabla P|\,\delta/4\eta_c = 3U_{av}/\delta$, which coincides with the definition (4). Going back to the non-Newtonian problem, the average velocity $U_{av}$ of a fluid flowing along a rectangular channel of width $W$ and height $H$, is given by the known flow rate $Q_c$

$$U_{av} = \frac{Q_c}{WH}. \tag{5}$$

This allows to determine $\dot\gamma_{\mathrm{eff}}$ based on (4)-(5). The corresponding value of the viscosity can be computed by the power-law fluid model

$$\eta(\dot\gamma) = K\,\dot\gamma^{\,(n-1)}. \tag{6}$$

The following simple (dimensional) argument suggests that further dimensionless refinements with respect to Eq. (3) [6] can be introduced. Indeed, the equations of motion for a viscous fluid in presence of thinning effects would balance the viscous forces with the pressure-driven forces as $\boldsymbol{\nabla}\cdot(\eta_c(\dot{\gamma})\boldsymbol{\nabla u}) = \boldsymbol{\nabla} P$. We then find $(\boldsymbol{\nabla}\eta_c(\dot{\gamma}))\cdot\boldsymbol{\nabla u}+\eta_c(\dot{\gamma})\nabla^2\boldsymbol{u} = \boldsymbol{\nabla} P$. For a Newtonian fluid, $\boldsymbol{\nabla}\eta_c(\dot{\gamma}) = 0$, and the definition of Capillary number (2) would obviously be recovered from the usual balancing of $\eta_c\nabla^2\boldsymbol{u}$ and $\boldsymbol{\nabla} P$. In presence of thinning contributions, one has to account for the term $(\boldsymbol{\nabla}\eta_c(\dot{\gamma}))\cdot\boldsymbol{\nabla u}$. A simple dimensional estimate gives $\boldsymbol{\nabla}\eta_c(\dot{\gamma}) \approx \partial\eta_c/\partial\dot{\gamma}\,\nabla^2\boldsymbol{u} = (n-1)\frac{\eta_c(\dot{\gamma})}{\dot{\gamma}}\nabla^2\boldsymbol{u}$, hence $(\boldsymbol{\nabla}\eta_c(\dot{\gamma}))\cdot\boldsymbol{\nabla u} \approx (n-1)\eta_c(\dot{\gamma})\boldsymbol{\nabla}^2\boldsymbol{u}$. Thus, by thinking of a small gradient expansion around $\dot{\gamma} \approx \dot{\gamma}_{\text{eff}}$, one can approximate the viscous contributions as $\boldsymbol{\nabla}\cdot(\eta_c(\dot{\gamma})\boldsymbol{\nabla u}) \approx n\eta_c(\dot{\gamma}_{\text{eff}})\nabla^2\boldsymbol{u}$. This argument suggests that beyond the definition (3), a better accounting of the thinning effects comes from the redefinition:

$$\overline{\mathrm{Ca}} = n\,\mathrm{Ca}_{\text{eff}} \tag{7}$$

$n$ being the flow behaviour of the power-law fluid. This definition has been used to rescale the data of Fig. 3 in the manuscript.

## IV. BREAKUP MAPS

The panels of Fig. S1 report the *breakup maps* for all the data shown in Fig. 2 of the manuscript, i.e. the different symbols indicate whether the breakup occurs in squeezing (S), dripping (D) or jetting (J). The data refer only to values of $\varphi$ and $Q_c$ for which droplet formation is stable and occurs at the T-junction. Production at other $\varphi$ and $Q_c$ is either not stable (low $\varphi$, $Q_c$), or out of reach of the experimental setup. The transition to jetting is characterised by particular values ${Q_c}^*$ of the continuous flow rate that depend on $\varphi$. These are identified by analyzing the evolution of droplet breakup, at fixed $\varphi$ and increasing $Q_c$, as shown in panel (F). The left and right snapshots refer, respectively, to the instant just before and just after breakup for a typical sequence. At low $Q_c$ the breakup takes place at the corner of the T-junction and after the droplet detachment the tip of the dispersed phase returns back into the side channel (1). At higher $Q_c$ the breakup starts to take place after the corner and the tip returns back stopping at the level of the corner of the T-junction (3) and then oversteps it (4) persisting in the main channel. At even larger $Q_c$, the dispersed phase starts to jet (6). As the transition is continuous over a range of $Q_c$, the delimiting value ${Q_c}^*$ is chosen to be the one at which, just after breakup, the tip of the dispersed phase oversteps the corner of the T-junction, as indicated in the figure. The breakup maps are observed to be strongly dependent on $\lambda$. Overall, for lower $\lambda$ the transition is shifted to higher $Q_c$. In particular, for the lowest $\lambda \sim 0.3$ (Fig. S1-E) the transition is observed at $Q_c$ higher than the ones accessible by the acquisition system, and thus can not be measured accurately.

## V. RHEOLOGY OF XANTHAN SOLUTIONS

In Fig. S2 we recall the essential features of the rheological characterization [7] of the Xanthan solutions used as continuous phase in the droplets breakup, performed by a parallel plate rheometer (Advanced Rheometric Expansion System ARES, TA instruments). As extensively addressed by [6–8], although Xanthan is a well established model system for shear thinning fluids, a weak elastic response of the polymer solutions starts emerging in the semi dilute regime. Three different concentrations are used to study the droplet breakup in polymer solutions. Only for Xanthan concentrated at 1500 ppm a first normal stress difference $N_1$ is measurable, whereas at lower Xanthan concentration $N_1$ is so small to result undetectable by the rheometer. To assess a possible importance of the emergent normal stress showed in Fig. S2 LBM simulations are performed with pure thinning phases (see Sec. III of the manuscript)

## VI. NUMERICAL SIMULATIONS

### A. Lattice Boltzmann for purely shear thinning liquids

Thanks to the LBM, we are able to reproduce the NS hydrodynamic equations for both Newtonian [9] and shear thinning fluids [7, 10]. Specifically, in the carrier (c) and dispersed (d) phases the following continuum equations are integrated:

$$\rho_{c,d}\left[\partial_t\boldsymbol{u}_{c,d} + (\boldsymbol{u}_{c,d}\cdot\boldsymbol{\nabla})\boldsymbol{u}_{c,d}\right] = -\boldsymbol{\nabla} P_{c,d} + \boldsymbol{\nabla}\left(\eta_{c,d}(\boldsymbol{\nabla u}_{c,d} + (\boldsymbol{\nabla u}_{c,d})^T)\right) \tag{8}$$

where the hydrodynamic velocity and the dynamic viscosity are indicated with $\boldsymbol{u}_{c,d}$ and $\eta_{c,d}$, respectively. The superscript $T$ indicates the transpose of the gradient tensor. The density and bulk pressure are indicated with $\rho_{c,d}$

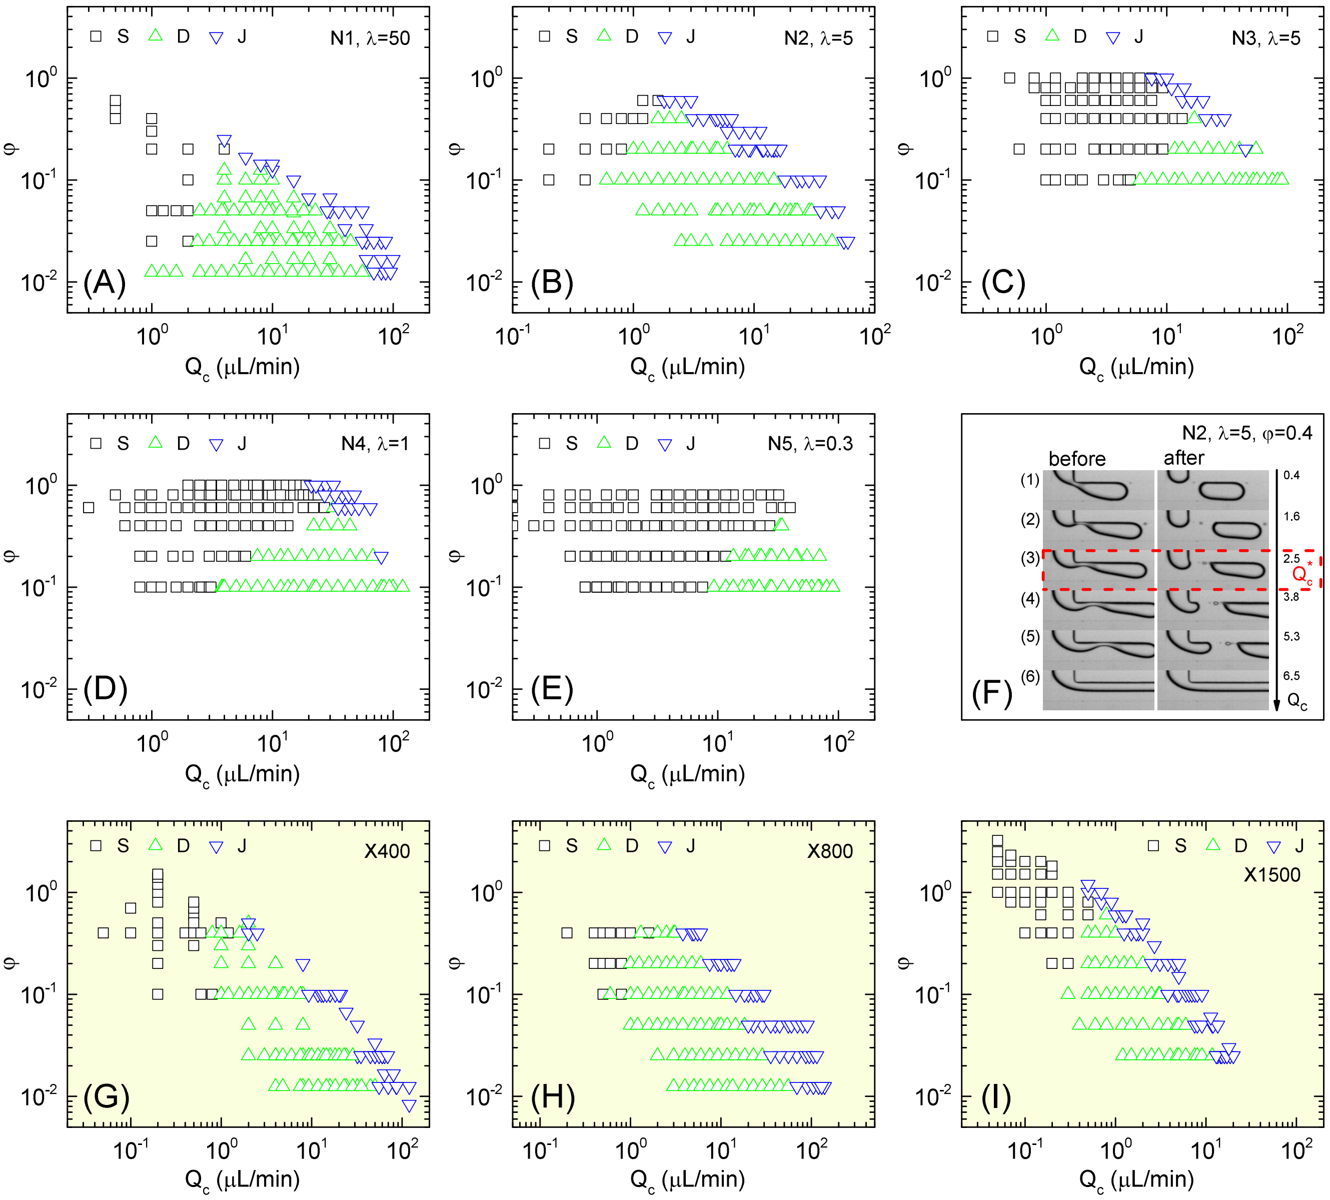


FIG. S1. Panels (A)-(E) show the breakup maps of the Newtonian systems for all the combination of $\varphi$ and $Q_c$ investigated, reporting whether the breakup occurs in squeezing (S), dripping (D) or jetting (J). Similarly, panels (G)-(I) report the breakup maps for the non-Newtonian systems. Close to the transition to jetting, the data are marked as jetting when, at a fixed $\varphi$, the value of $Q_c \geq Q_c{}^*$. The value $Q_c{}^*$ of the continuous flow rate corresponding to the transition to the jetting regime is described in the snapshots in panel (F). The left and right snapshots correspond to the time just before and just after breakup, respectively, at a fixed $\varphi$ and increasing $Q_c$ (from top to bottom) for a typical experiment (N2, $\varphi = 0.4$ is shown). The value of $Q_c{}^*$ is chosen to be the minimum $Q_c$ at which, just after breakup, the tip of the dispersed phase remains inside the main channel, as indicated in the snapshots. Panel (E) does not report the jetting, as the corresponding flow rates are out the reach of the experimental setup.

and $P_{c,d}$. In the continuous phase, the viscosity is chosen to be

$$\eta_c(\dot\gamma) = \begin{cases} \eta_0 + K\dot\gamma_0^{n-1} & \dot\gamma \leq \dot\gamma_0 \\ \eta_0 + K\dot\gamma^{n-1} & \dot\gamma > \dot\gamma_0 \end{cases} \tag{9}$$

where $K = 0.05$ (lbu, lattice Boltzmann units hereafter) and where the cut-off $\dot\gamma_0 = 10^{-5}$ lbu is introduced to cure viscosity divergence at small shear rates [7]. Thinning effects are included by using LBM relaxation times which depend on the local shear rate, as explained in [10], hence we do not consider any explicit polymer dynamics [11, 12].

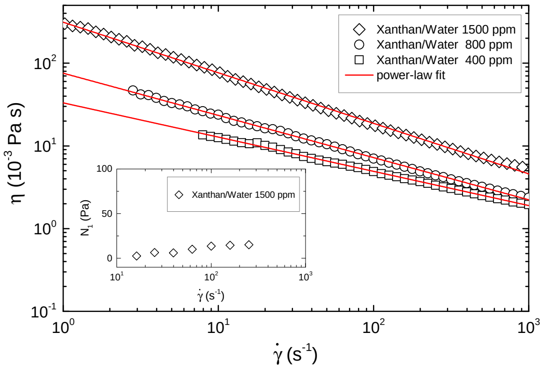


FIG. S2. Rheological characterization of Xanthan solutions as a function of the shear rate for different concentration of Xanthan in water. Main graph: shear dependent viscosity for different concentrations; lines are best fit to the experimental data accordingly to the power-law fluid model described in Eq. (6). Inset: first normal stress difference for the most concentrated Xanthan solution. The Xanthan data of both $N_1$ and $\eta$ are reproduced from [7] with kind permission of The European Physical Journal (EPJ).

The background viscosity $\eta_0 = 0.3$ lbu is introduced to avoid a zero viscosity and numerical instabilities in the limit of high shear rates. In the dispersed phase, the viscosity is kept constant to $\eta_d = \eta_0 = 0.3$ lbu so that the viscosity ratio between the dispersed and the continuous phase falls in the interval $[0.1 - 1]$ for the thinning exponents considered ($n \in [0.7 : 1.0]$). Smaller values of $n$ are not easily handled in the numerical simulations, due to the larger viscous ratio associated with them and the numerical instabilities encountered. Table S1 summarizes all the parameters used in our numerical investigations for both Newtonian and non Newtonian phases. Different numerical resolutions are adopted to resolve the channels. A single numerical simulation (i.e. fixed Ca or $\overline{\mathrm{Ca}}$) requires between 1 and 3 days on a multiprocessor cluster comprising of 512 cores.

| Ca | $\varphi$ | $n$ |
|---|---|---|
| $0.001 - 0.1$ | 0.5 | 1.0, 0.9, 0.8, 0.75, 0.7 |
| $0.001 - 0.1$ | 1.0 | 1.0, 0.9, 0.8, 0.75, 0.7 |

TABLE S1. Parameters for the numerical simulations with the T-junction geometry for thinning fluid.

### B. Numerical Benchmark for Newtonian liquids

LBM simulations are compared with experiments performed with purely Newtonian fluids, i.e. $\eta_c =$ const. in Eq. (9). Corresponding results are reported in Fig. S3. They display behaviours that quantitatively agree with the experimental data in the time dynamics of the breakup process. Specifically, in panels (A-H) we report a representative case corresponding to $\mathrm{Ca} = 0.0085$, $\varphi = 0.4$ and $\lambda = 1.0$, where the system is switching from the squeezing dominated regime to the dripping regime. The process of droplet formation comes out to be in good agreement with both experiments and numerical simulations. To make time dimensionless we have used the characteristic shear time $\tau_{\mathrm{shear}} = W/U_{av}$ as a unit of time. More quantitatively, for a fixed $\varphi$, the droplet size is a decreasing function of Ca (see Panel (I)); moreover, for a fixed Ca, one reproduces a linear scaling law for the droplet size as a function of $\varphi$ (see inset). We generically observed that for Capillary numbers $\mathrm{Ca} \approx \mathcal{O}(10^{-2})$ the droplet size is well in agreement with the experimental results, and only a slight mismatch emerges at higher Ca [13, 14], in the jetting regime, which is however not of interest for the present study. Overall, the simulations of Newtonian fluids retain the key relevant outcomes of the experiments, in terms of droplet size behaviour as a function of Ca and $\varphi$. Hence, they are good candidates to explore quantitatively the effects solely induced by the thinning behaviour as well as the validity of the rescaling properties at changing both Ca, $n$ and $\varphi$. This analysis, in conjunction with the experimental results, is presented in the text.

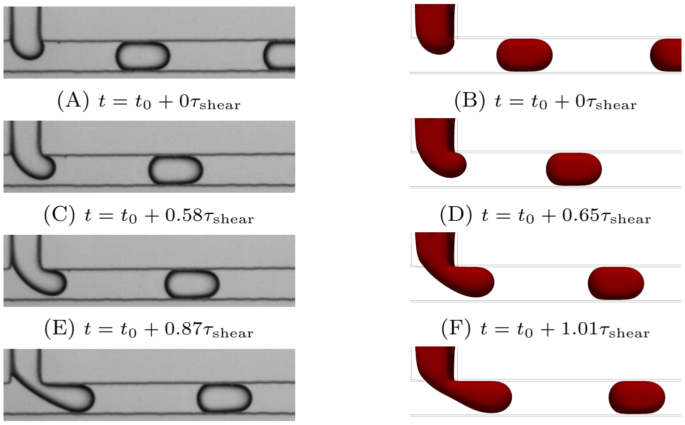

(A) $t = t_0 + 0\tau_{\text{shear}}$ (B) $t = t_0 + 0\tau_{\text{shear}}$

(C) $t = t_0 + 0.58\tau_{\text{shear}}$ (D) $t = t_0 + 0.65\tau_{\text{shear}}$

(E) $t = t_0 + 0.87\tau_{\text{shear}}$ (F) $t = t_0 + 1.01\tau_{\text{shear}}$

(G) $t = t_0 + 1.45\tau_{\text{shear}}$ (H) $t = t_0 + 1.50\tau_{\text{shear}}$

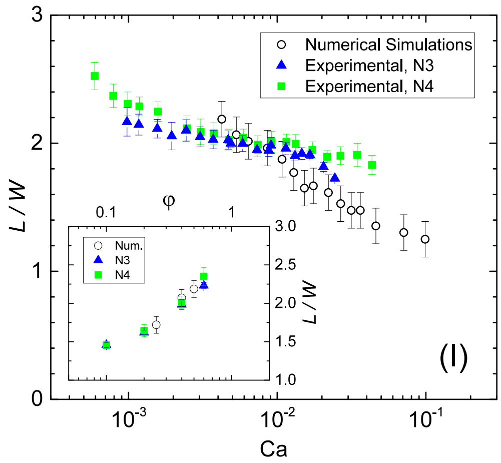


FIG. S3. Panels (A-H): time dynamics for the droplet formation process in the squeezing-to-dripping transition from experiments (left snapshots) and LBM simulations (right snapshots) for Ca = 0.0085, $\varphi = 0.4$ and $\lambda = 1.0$. Time is made dimensionless using the shear time $\tau_{\text{shear}} = W/U_{av}$. Panel (I): quantitative comparison between the numerical simulations and the experiments for the normalized droplet size as a function of the Capillary number. The inset reports data for a fixed Capillary number Ca = 0.008 for different Newtonian continuous phases (only fluids N3 and N4 are shown, see Table II of the manuscript for details).


[1] J. C. McDonald and G. M. Whitesides, "Poly(dimethylsiloxane) as a material for fabricating microfluidic devices," Accounts of Chemical Research **35**, 491 (2002).
[2] T. Tóth, D. Ferraro, E. Chiarello, M. Pierno, G. Mistura, G. Bissacco, and C. Semprebon, "Suspension of water droplets on individual pillars," Langmuir **27**, 4742 (2011).
[3] S. K. Sia and G. M. Whitesides, "Microfluidic devices fabricated in poly (dimethylsiloxane) for biological studies," Electrophoresis **24**, 3563 (2003).
[4] E. Chiarello, L. Derzsi, M. Pierno, G. Mistura, and E. Piccin, "Generation of oil droplets in a non-newtonian liquid using a microfluidic t-junction," Micromachines **6**, 1825 (2015).
[5] G. F. Christopher, N. N. Noharuddin, J. A. Taylor, and S. L. Anna, "Experimental observations of the squeezing-to-dripping transition in T-shaped microfluidic junctions," Physical Review E **78**, 036317 (2008).
[6] S. Varagnolo, D. Filippi, G. Mistura, M. Pierno, and M. Sbragaglia, "Stretching of viscoelastic drops in steady sliding," Soft Matter **13**, 3116 (2017).
[7] S. Varagnolo, M. Pierno, G. Mistura, and M. Sbragaglia, "Sliding droplets of xanthan solutions: a joint experimental and numerical study," The European Physical Journal E **38**, 126 (2015).
[8] C. W. Macosko, *Rheology: principles, measurements, and applications* (Wiley-VCH, Berlin, 1994).
[9] S. Succi, *The Lattice Boltzmann Equation for Fluid Dynamics and Beyond* (Oxford University Press, 2001).
[10] S. Gabbanelli, G. Drazer, and J. Koplik, "Lattice boltzmann method for non-newtonian (power-law) fluids," Physical Review E **72**, 046312 (2005).
[11] A. Gupta and M. Sbragaglia, "Effects of viscoelasticity on droplet dynamics and break-up in microfluidic t-junctions: a lattice boltzmann study," The European Physical Journal E **39**, 6 (2016).
[12] A. Gupta and M. Sbragaglia, "A lattice boltzmann study of the effects of viscoelasticity on droplet formation in microfluidic cross-junctions," The European Physical Journal E **39**, 2 (2016).
[13] M. Sbragaglia, L. Biferale, G. Amati, S. Varagnolo, D. Ferraro, G. Mistura, and M. Pierno, "Sliding drops across alternating hydrophobic and hydrophilic stripes," Physical Review E **89**, 012406 (2014).
[14] H. Kusumaatmaja, J. Leopoldes, A. Dupuis, and J. Yeomans, "Drop dynamics on chemically patterned surfaces," Europhysics Letters **73**, 740 (2006).
